# Supplementary material for: Heat rectification via a superconducting artificial atom
Source: arXiv:1908.05574 source file (2019-08-16)
Supplement: Supplementary file 1 [file HeatRect_SI.pdf]

# Supplementary material

(Dated: August 15, 2019)

## I. RECTIFICATION IN A TWO-LEVEL SYSTEM

### A. Qubit

Consider a qubit coupled to two baths as shown in Fig. 1a. The transition rates are given by

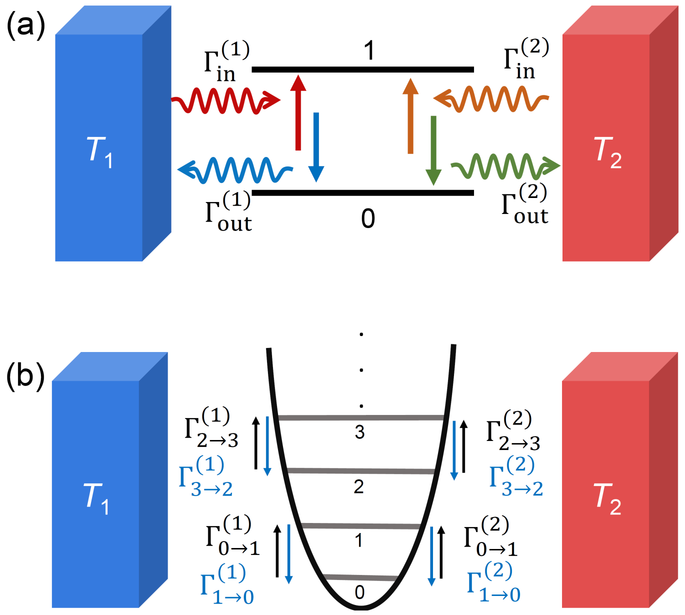


FIG. 1: (a) A two-level system coupled to two baths, together with the associated transition rates. (b) As (a) but qubit replaced by a harmonic oscillator.

$$\Gamma_{\text{in}}^{(1)} = g_1 \frac{\omega_{\text{q}}}{e^{\beta_1 \hbar\omega_{\text{q}}} - 1}, \qquad \Gamma_{\text{in}}^{(2)} = g_2 \frac{\omega_{\text{q}}}{e^{\beta_2 \hbar\omega_{\text{q}}} - 1}$$
$$\Gamma_{\text{out}}^{(1)} = g_1 \frac{\omega_{\text{q}}}{1 - e^{-\beta_1 \hbar\omega_{\text{q}}}}, \qquad \Gamma_{\text{out}}^{(2)} = g_2 \frac{\omega_{\text{q}}}{1 - e^{-\beta_2 \hbar\omega_{\text{q}}}}, \tag{1}$$

where $g_i$ is the coupling to bath $i = 1, 2$, $\hbar\omega_{\text{q}}$ denotes the energy level separation of the qubit, and $\beta_i = 1/k_{\text{B}}T_i$ is the inverse temperature of each bath. In steady state the population of the excited state, $\rho_e = 1 - \rho_g$ reads

$$\rho_e = \frac{\Gamma_{\text{in}}}{\Gamma_{\text{in}} + \Gamma_{\text{out}}}, \tag{2}$$

where $\Gamma_{\text{in,out}} = \Gamma_{\text{in,out}}^{(1)} + \Gamma_{\text{in,out}}^{(2)}$ and $\rho_g$ is the population of the ground state of the qubit. The expression for power to bath $i$ is then

$$P_i = \hbar\omega_{\text{q}}(\rho_e \Gamma_{\text{out}}^{(i)} - \rho_g \Gamma_{\text{in}}^{(i)}). \tag{3}$$

The thermal rectification by definition is given by

$$\mathcal{R} = |\frac{P_i^+}{P_i^-}|, \tag{4}$$

where $\pm$ refers to the sign of the temperature bias. Consider case when one of the bath temperatures is much smaller than the other with $k_{\text{B}}T = 1/\beta$ the higher temperature. In this case the rectification ratio is given by

$$\mathcal{R} = \frac{g_1 + g_2 \coth(\frac{\beta\hbar\omega_{\text{q}}}{2})}{g_1 \coth(\frac{\beta\hbar\omega_{\text{q}}}{2}) + g_2}. \tag{5}$$

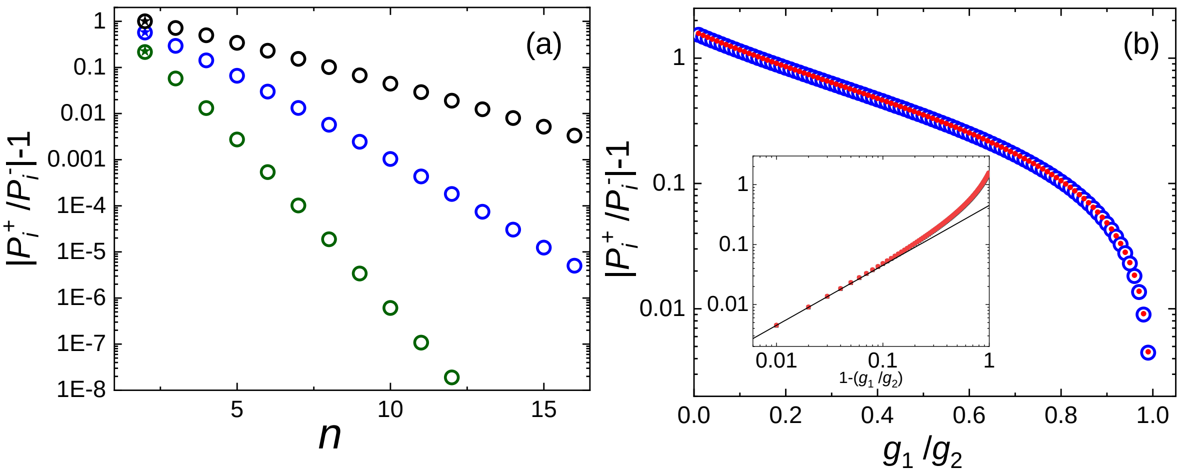


FIG. 2: Rectification ratio. (a) $\mathcal{R}-1$ versus number of levels $n$. The parameters are: $g_1/g_2 = 1/3$, black circles $\beta_1\hbar\omega_q = 0.4$ and $\beta_2\hbar\omega_q = 4.8$, blue circles $\beta_1\hbar\omega_q = 0.8$ and $\beta_2\hbar\omega_q = 4.8$, and green circles $\beta_1\hbar\omega_q = 1.6$ and $\beta_2\hbar\omega_q = 4.8$. Stars at $n = 2$ are from Eq. (4). (b) $\mathcal{R}-1$ versus asymmetry for $n = 2$. Blue circles are from the numerics and red ones from Eq. (4). The parameters are: $\beta_1\hbar\omega_q = 0.8$ and $\beta_2\hbar\omega_q = 4.8$.

For small asymmetry $\delta = 1 - g_1/g_2$, $|\delta| \ll 1$, one can expand the rectification ratio into

$$\mathcal{R} - 1 = e^{-\beta\hbar\omega_q}\delta. \tag{6}$$

The inset of Fig. 2b shows this result by solid line for the corresponding temperature.

## II. MULTILEVEL SYSTEM

Consider $n$-level system with constant energy spacing $\hbar\omega_q$. In the limit of $n \to \infty$ it represents a linear harmonic oscillator as shown in Fig. 1b. The transition rates between levels $k$ and $k \pm 1$ are given by

$$\Gamma^{(i)}_{k\to k\pm1} = \frac{1}{\hbar^2}|\langle k|\hat{Q}|k\pm1\rangle|^2 S_i(\mp\omega_q). \tag{7}$$

Here $i = 1, 2$ refers to the baths, $\hat{Q} = i\sqrt{\frac{\hbar}{2Z_0}}(\hat{a}^\dagger - \hat{a})$ and $S_i(\omega) = 2R_i\frac{\hbar\omega}{1-e^{-\beta_i\hbar\omega}}$ are charge operator and voltage noise when applied to a circuit, respectively. Here, $Z_0$ is a characteristic impedance of the system, $\hat{a}$ ($\hat{a}^\dagger$) is annihilation (creation) operator of the ladder of the system, and $R_i$ is the resistance of the bath. In this case only the transitions between the nearest levels are allowed according to

$$\Gamma^{(i)}_{k\to k-1} = k\Gamma^{(i)}_{\text{out}}$$
$$\Gamma^{(i)}_{k-1\to k} = k\Gamma^{(i)}_{\text{in}}. \tag{8}$$

The steady state population of each level reads $\rho_i = S_i/S$, where

$$S_0 = \prod_{k=1}^{n}\Gamma_{k\to k-1}, \quad S_j = \prod_{k=1}^{j}\Gamma_{k-1\to k}\prod_{k=j+1}^{n}\Gamma_{k\to k-1}, \quad S_n = \prod_{k=1}^{n}\Gamma_{k-1\to k}, \quad S = \sum_{i=0}^{n} S_i, \tag{9}$$

where $1 \le j \le n-1$ and $\Gamma_{k\to k\pm1} = \Gamma^{(1)}_{k\to k\pm1} + \Gamma^{(2)}_{k\to k\pm1}$. The expression of power to bath $i$ is then given by

$$P_i = \hbar\omega_q\sum_{k=1}^{n}(\Gamma^{(i)}_{k\to k-1}\rho_k - \Gamma^{(i)}_{k-1\to k}\rho_{k-1}). \tag{10}$$

As seen in Fig. 2a, the rectification vanishes exponentially when the number of equidistant levels increases.

## III. ENERGY LEVELS OF THE EXPERIMENTAL DEVICE

The Hamiltonian $\hat{H}$ is given by

$$\hat{H} = \hbar\omega_{\rm L}\hat{a}_{\rm L}^\dagger\hat{a}_{\rm L} + \hbar\omega_{\rm q}\hat{a}_{\rm q}^\dagger\hat{a}_{\rm q} + \hbar\omega_{\rm R}\hat{a}_{\rm R}^\dagger\hat{a}_{\rm R} + g(\hat{a}_{\rm q}\hat{a}_{\rm L}^\dagger + \hat{a}_{\rm q}^\dagger\hat{a}_{\rm L} + \hat{a}_{\rm q}\hat{a}_{\rm R}^\dagger + \hat{a}_{\rm q}^\dagger\hat{a}_{\rm R}) + \tilde{g}(\hat{a}_{\rm L}\hat{a}_{\rm R}^\dagger + \hat{a}_{\rm L}^\dagger\hat{a}_{\rm R}). \tag{11}$$

Here, $\hbar\omega_{\rm L}$, $\hbar\omega_{\rm q}$, and $\hbar\omega_{\rm R}$ are the energies of the left resonator, qubit and the right resonator, respectively, $g$ is the common coupling constant of the qubit to the two resonators, and $\tilde{g}$ is the cross-coupling between the resonators. In the eleven-level basis of $|000\rangle$, $|100\rangle$, $|010\rangle$, $|001\rangle$, $|110\rangle$, $|101\rangle$, $|011\rangle$, $|111\rangle$, $|200\rangle$, $|210\rangle$, $|300\rangle$, $|310\rangle$, where the entries in each state refer to the left resonator, the qubit, and the right resonator, respectively, the matrix form of the Hamiltonian can be written

$$H = \hbar\omega_0 \begin{pmatrix} 0 & 0 & 0 & 0 & 0 & 0 & 0 & 0 & 0 & 0 & 0 \\ 0 & 1-a/2 & \gamma & \tilde{\gamma} & 0 & 0 & 0 & 0 & 0 & 0 & 0 \\ 0 & \gamma & r & \gamma & 0 & 0 & 0 & 0 & 0 & 0 & 0 \\ 0 & \tilde{\gamma} & \gamma & 1+a/2 & 0 & 0 & 0 & 0 & 0 & 0 & 0 \\ 0 & 0 & 0 & 0 & 1-a/2+r & \gamma & \tilde{\gamma} & 0 & \sqrt{2}\gamma & 0 & 0 \\ 0 & 0 & 0 & 0 & \gamma & 2 & \gamma & 0 & \sqrt{2}\tilde{\gamma} & 0 & 0 \\ 0 & 0 & 0 & 0 & \tilde{\gamma} & \gamma & r+1+a/2 & 0 & 0 & 0 & 0 \\ 0 & 0 & 0 & 0 & 0 & 0 & 0 & 2+r & 0 & \sqrt{2}\tilde{\gamma} & 0 \\ 0 & 0 & 0 & 0 & \sqrt{2}\gamma & \sqrt{2}\tilde{\gamma} & 0 & 0 & 2-a & 0 & 0 \\ 0 & 0 & 0 & 0 & 0 & 0 & 0 & \sqrt{2}\tilde{\gamma} & 0 & 2-a+r & \sqrt{3}\gamma \\ 0 & 0 & 0 & 0 & 0 & 0 & 0 & 0 & 0 & \sqrt{3}\gamma & 3-3a/2 \end{pmatrix}, \tag{12}$$

where $\omega_0 = \frac{\omega_{\rm R}+\omega_{\rm L}}{2}$, $a = \frac{\omega_{\rm R}-\omega_{\rm L}}{\omega_0}$, $\gamma = \frac{g}{\hbar\omega_0}$, $\tilde{\gamma} = \frac{\tilde{g}}{\hbar\omega_0}$, and $r = \frac{\hbar\omega_{\rm q}}{\hbar\omega_0}$. Here $\omega_{\rm L} = 2\pi \times 2.8$ GHz and $\omega_{\rm R} = 2\pi \times 6.5$ GHz are constant, and $\hbar\omega_q = \sqrt{8E_J E_C|\cos(\pi\Phi/\Phi_0)|} - E_{\rm C}$ like in the anharmonic Josephson potential.

## IV. STATISTICS AND RECTIFICATION

Rectification (in a two-level system) depends on the statistics of transition rates. In particular let us consider fermions vs bosons. The latter case was discussed earlier in this Supplementary Material.

We may write the transition rate into the system via contact $i$ for fermions (+) and bosons (-) as

$$\Gamma_{\rm in}^{(i)} = g_i \frac{1}{e^{\beta_i E} \pm 1}. \tag{13}$$

For fermions, we may take a single level quantum dot, where $g_i$ is determined by the barrier, and $E$ is the energy level position of the dot with respect to the fermi level, controlled by gate as shown in Fig. 3a. For bosons, we may take as above a qubit coupled to a dissipative environment: $g_i = \omega_0/Q_i$, where $E = \hbar\omega_{\rm q}$ is the level splitting of the qubit, and $Q_i$ the quality factor of the environment $i$ (Fig. 3b). For both cases, the detailed balance condition holds

$$\Gamma_{\rm out}^{(i)} = e^{\beta_i E}\Gamma_{\rm in}^{(i)} \tag{14}$$

for the rate out from the system.

Steady-state occupation on the excited state of the system is given by

$$\rho_e = \frac{\Gamma_{\rm in}^{(1)} + \Gamma_{\rm in}^{(2)}}{\Gamma_{\rm in}^{(1)} + \Gamma_{\rm in}^{(2)} + \Gamma_{\rm out}^{(1)} + \Gamma_{\rm out}^{(2)}}. \tag{15}$$

Let us assume for simplicity that bath 1 has inverse temperature $\beta$ and bath 2 is at zero temperature. Then we find the power to bath 2 as

$$P_2 = \rho_e E \Gamma_{\rm out}^{(2)}. \tag{16}$$

For fermions we find

$$P_2 = \frac{g_1 g_2}{g_1 + g_2} E f(E), \tag{17}$$

where $f(E) = 1/(e^{\beta E} + 1)$. Due to the symmetry with respect to indices 1 and 2, this system does not rectify heat. On the contrary, as we saw already earlier, for bosons the situation is different, and we obtain

$$P_2 = \frac{g_1 g_2}{g_1 \coth(\beta E/2) + g_2} E n(E), \tag{18}$$

where $n(E) = 1/(e^{\beta E} - 1)$. This expression yields rectification when $g_1 \neq g_2$.

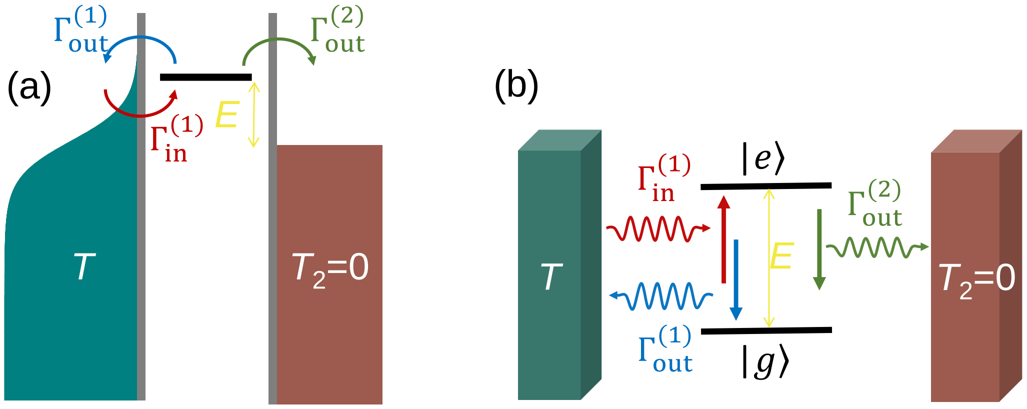


FIG. 3: Single-level quantum dot in (a) and a qubit in (b).
